# Supplementary material for: Collaborative Face Experts Fusion in Video Generation: Boosting Identity Consistency Across Large Face Poses
Source: arXiv:2508.09476 source file (2025-12-05)
Supplement: Supplementary file 1 [file visual_abla_suppl.tex]

\begin{figure}[t]
    \centering
    \includegraphics[width=\linewidth]{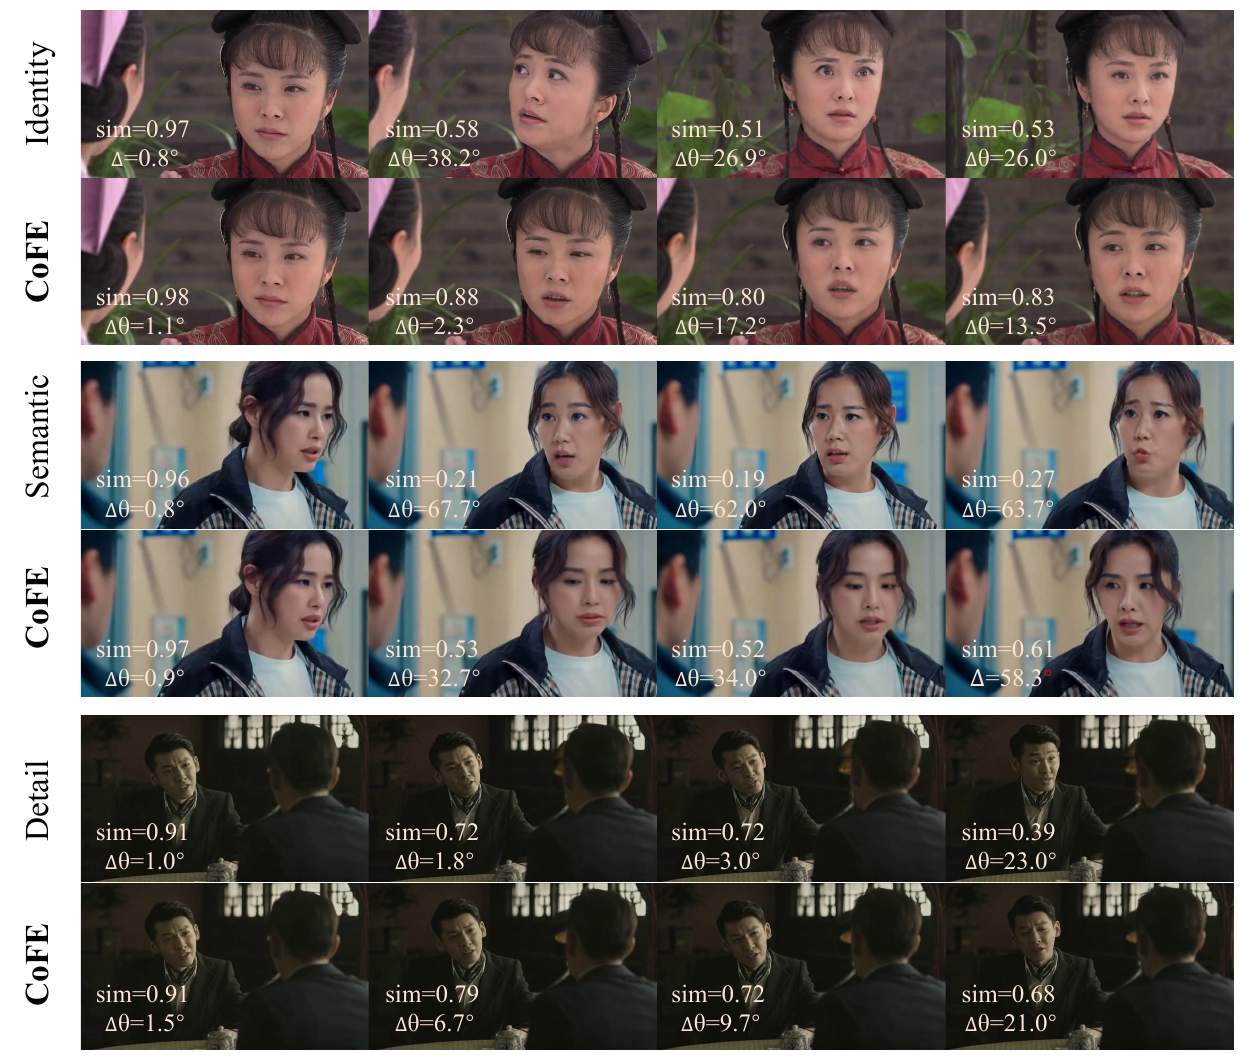}
    \caption{Detailed comparison of different feature injections.}
    \label{fig:visual_abla_suppl}
\end{figure}
